# Supplementary material for: A realizability-preserving high-order kinetic scheme using WENO reconstruction for entropy-based moment closures of linear kinetic equations in slab geometry
Source: arXiv:1501.07765 source file (2015-06-26)
Supplement: Supplementary file 1 [file supp-mis.tex]

% This file is not needed, for instance supp-pdf has the relevant code
% built in and ppchtex is adapted.

\input supp-mis.mkii
